# Supplementary material for: Assessing the accuracy of direct-coupling analysis for RNA contact prediction
Source: arXiv:1812.07630 ancillary file (2019-11-29)
Supplement: Supplementary file 1 [file si.pdf]

# Supporting Information

Francesca Cuturello [1], Guido Tiana [2], Giovanni Bussi [1]

December 18, 2018

Table 1: PDB, RFAMcode molecule name, alignment length and size, effective alignment size after reweighting of the data set.

| **PDB** | **RFAM** | **molecule name** | **length** | **size** | **size$_{\mathbf{eff}}$** |
|---|---|---|---|---|---|
| 4L81 | RF01725 | SAM-I/IV variant riboswitch | 97 | 693 | 128 |
| 2GDI | RF00059 | TPP riboswitch | 80 | 10858 | 1054 |
| 3F2Q | RF00050 | FMN riboswitch | 109 | 3144 | 1078 |
| 2GIS | RF00162 | SAM riboswitch | 93 | 4903 | 910 |
| 1Y26 | RF00167 | Purine riboswitch | 71 | 2589 | 508 |
| 3DOU | RF00168 | Lysine riboswitch | 161 | 1870 | 832 |
| 4QLM | RF00379 | ydaO/yuaA leader | 108 | 2723 | 1067 |
| 2QBZ | RF00380 | ykoK leader | 153 | 850 | 240 |
| 5T83 | RF00442 | ykkC-yxkD leader | 89 | 687 | 138 |
| 3OWI | RF00504 | Glycine riboswitch | 88 | 4602 | 985 |
| 3IRW | RF01051 | Cyclic di-GMP-I riboswitch | 91 | 2231 | 578 |
| 4FRG | RF01689 | AdoCbl variant RNA | 84 | 189 | 25 |
| 3VRS | RF01734 | Fluoride riboswitch | 52 | 1426 | 312 |
| 5DDP | RF01739 | Glutamine riboswitch | 61 | 1138 | 179 |
| 4XW7 | RF01750 | ZMP/ZTP riboswitch | 64 | 1197 | 432 |
| 3SD3 | RF01831 | THF riboswitch | 89 | 547 | 205 |
| 4RUM | RF02683 | NiCo riboswitch | 92 | 207 | 42 |

Table 2: $\overline{MCC}$ with optimal covariance score threshold $\overline{S}$ for Boltzmann learning DCA, pseudo-likelihood DCA, mean field DCA, mutual information for each of 17 RNA families, obtained through cross-validation procedure. Alignments are performed with *Infernal*.

| | **Boltzmann learning DCA** | | **Pseudo-likelihood DCA** | | **mean field DCA** | | **mutual information** | |
|---|---|---|---|---|---|---|---|---|
| PDB | $\overline{MCC}$ | $\overline{S}$ | $\overline{MCC}$ | $\overline{S}$ | $\overline{MCC}$ | $\overline{S}$ | $\overline{MCC}$ | $\overline{S}$ |
| 3DOU | 0.68 | 1.09 | 0.59 | 0.65 | 0.67 | 1.0 | 0.68 | 0.22 |
| 3F2Q | 0.58 | 1.09 | 0.58 | 0.65 | 0.56 | 1.0 | 0.55 | 0.22 |
| 2QBZ | 0.55 | 1.09 | 0.50 | 0.78 | 0.52 | 1.0 | 0.53 | 0.22 |
| 2GDI | 0.55 | 1.09 | 0.51 | 0.65 | 0.57 | 1.0 | 0.48 | 0.22 |
| 1Y26 | 0.69 | 1.09 | 0.67 | 0.65 | 0.63 | 0.99 | 0.63 | 0.22 |
| 5T83 | 0.58 | 1.09 | 0.58 | 0.65 | 0.58 | 1.0 | 0.53 | 0.22 |
| 5DDP | 0.65 | 1.09 | 0.63 | 0.65 | 0.66 | 1.0 | 0.65 | 0.22 |
| 4XW7 | 0.59 | 1.24 | 0.63 | 0.65 | 0.59 | 1.0 | 0.55 | 0.22 |
| 4RUM | 0.60 | 1.19 | 0.39 | 0.78 | 0.54 | 1.06 | 0.55 | 0.22 |
| 4L81 | 0.46 | 1.09 | 0.45 | 0.78 | 0.43 | 1.0 | 0.35 | 0.22 |
| 4FRG | 0.63 | 1.09 | 0.49 | 0.78 | 0.50 | 0.99 | 0.64 | 0.22 |
| 3SD3 | 0.67 | 1.05 | 0.69 | 0.65 | 0.67 | 1.0 | 0.63 | 0.22 |
| 2GIS | 0.67 | 1.14 | 0.74 | 0.65 | 0.44 | 1.03 | 0.37 | 0.22 |
| 3OWI | 0.73 | 1.11 | 0.73 | 0.65 | 0.67 | 1.0 | 0.29 | 0.24 |
| 3IRW | 0.58 | 1.09 | 0.56 | 0.65 | 0.50 | 1.0 | 0.35 | 0.22 |
| 4QLM | 0.56 | 1.05 | 0.58 | 0.65 | 0.49 | 1.0 | 0.43 | 0.22 |
| 3VRS | 0.64 | 1.11 | 0.71 | 0.65 | 0.71 | 1.0 | 0.67 | 0.22 |

Table 3: Clustal alignment. $\overline{MCC}$ with optimal covariance score threshold $\overline{S}$ for Boltzmann learning DCA, pseudo-likelihood DCA, mean field DCA, mutual information for each of 17 RNA families, obtained through cross-validation procedure.

| | **Boltzmann learning DCA** | | **Pseudo-likelihood DCA** | | **mean field DCA** | | **mutual information** | |
|---|---|---|---|---|---|---|---|---|
| PDB | $\overline{MCC}$ | $\overline{S}$ | $\overline{MCC}$ | $\overline{S}$ | $\overline{MCC}$ | $\overline{S}$ | $\overline{MCC}$ | $\overline{S}$ |
| 3DOU | 0.47 | 1.07 | 0.45 | 0.43 | 0.42 | 0.82 | 0.47 | 0.20 |
| 3F2Q | 0.48 | 0.99 | 0.45 | 0.43 | 0.32 | 0.80 | 0.31 | 0.20 |
| 2QBZ | 0.49 | 1.07 | 0.46 | 0.51 | 0.45 | 0.80 | 0.39 | 0.20 |
| 2GDI | 0.44 | 1.07 | 0.35 | 0.47 | 0.35 | 0.82 | 0.29 | 0.20 |
| 1Y26 | 0.57 | 1.07 | 0.50 | 0.43 | 0.51 | 0.82 | 0.32 | 0.20 |
| 5T83 | 0.41 | 1.07 | 0.38 | 0.43 | 0.32 | 0.82 | 0.44 | 0.20 |
| 5DDP | 0.42 | 1.10 | 0.33 | 0.51 | 0.19 | 0.82 | 0.20 | 0.20 |
| 4XW7 | 0.38 | 1.07 | 0.42 | 0.43 | 0.22 | 0.80 | 0.19 | 0.20 |
| 4RUM | 0.46 | 1.07 | 0.32 | 0.51 | 0.24 | 0.80 | 0.37 | 0.20 |
| 4L81 | 0.27 | 1.07 | 0.29 | 0.45 | 0.18 | 0.80 | 0.16 | 0.20 |
| 4FRG | 0.59 | 1.07 | 0.44 | 0.57 | 0.34 | 0.82 | 0.40 | 0.20 |
| 3SD3 | 0.71 | 1.07 | 0.72 | 0.45 | 0.58 | 0.8 | 0.50 | 0.20 |
| 2GIS | 0.54 | 0.99 | 0.54 | 0.43 | 0.40 | 0.82 | 0.34 | 0.20 |
| 3OWI | 0.42 | 1.07 | 0.48 | 0.47 | 0.40 | 0.82 | 0.24 | 0.20 |
| 3IRW | 0.55 | 1.07 | 0.37 | 0.44 | 0.39 | 0.80 | 0.25 | 0.20 |
| 4QLM | 0.38 | 1.07 | 0.45 | 0.51 | 0.30 | 0.80 | 0.10 | 0.23 |
| 3VRS | 0.55 | 1.08 | 0.42 | 0.43 | 0.42 | 0.82 | 0.34 | 0.20 |

Table 4: Average $\overline{MCC}$ at optimal covariance score threshold for DCA methods with and without APC correction. Alignments are performed with *Infernal*.

| | **Boltzmann learning DCA** | | **Pseudo-likelihood DCA** | | **mean field DCA** | |
|---|---|---|---|---|---|---|
| | APC | no APC | APC | no APC | APC | no APC |
| average $\overline{MCC}$ | 0.61 | 0.59 | 0.59 | 0.56 | 0.57 | 0.54 |

Table 5: Reweighting scheme: two sequences are considered similar if the fraction of positions with coincident nucleotides (*similarity*) is larger than a given similarity threshold $x$: $n_b = |s \in \{1, ..., B\} : similarity(\sigma^s, \sigma^b) > x|$. The inverse of $n_b$, $\omega_b = \frac{1}{n_b}$, gives a weight for the sequence contribution to frequencies ($B_{eff} = \sum_{b=1}^{B} \omega_b$ is then the effective number of sequences in the alignment). In this table we report the average $\overline{MCC}$ at optimal covariance score threshold for pseudo-likelihood DCA in the reweighting scheme adopting different similarity thresholds $x$. Alignments are performed with *Infernal*.

| | **x=0.7** | **x=0.8** | **x=0.9** | **x=1.0** |
|---|---|---|---|---|
| average $\overline{MCC}$ | 0.59 | 0.59 | 0.59 | 0.59 |

Table 6: Total stacked false positives (base atomes distance < 3.5 Å in the pdb reference structure) over total false positives for all methods. (*Infernal* alignment).

| | **Boltzmann learning** | **Pseudo-likelihood DCA** | **Mean Field** | **Mutual Information** |
|---|---|---|---|---|
| stacked FP / FP | 0.43 | 0.46 | 0.39 | 0.39 |

Table 7: $\overline{MCC}$ for each of 17 RNA families obtained through cross-validation procedure with optimal probability threshold $\overline{S}$. Base pairing probabilities are calculated from the RNAfold program available in the ViennaRNA package. We notice that for PDB 5T83 the MCC is zero for thresholds larger than ≈0.5, leading to a very low $\overline{S}$ whenever that system is included in the training set.

| PDB | $\overline{MCC}$ | $\overline{S}$ |
|---|---|---|
| 3DOU | 0.51 | 0.25 |
| 3F2Q | 0.52 | 0.25 |
| 2QBZ | 0.52 | 0.25 |
| 2GDI | 0.52 | 0.25 |
| 1Y26 | 0.51 | 0.25 |
| 5T83 | 0.58 | 0.72 |
| 5DDP | 0.51 | 0.25 |
| 4XW7 | 0.51 | 0.25 |
| 4RUM | 0.50 | 0.25 |
| 4L81 | 0.51 | 0.25 |
| 4FRG | 0.53 | 0.26 |
| 3SD3 | 0.52 | 0.25 |
| 2GIS | 0.51 | 0.25 |
| 3OWI | 0.50 | 0.25 |
| 3IRW | 0.53 | 0.25 |
| 4QLM | 0.52 | 0.25 |
| 3VRS | 0.54 | 0.25 |

**Algorithm 1** Boltzmann learning direct coupling analysis

1. **Initialization:**
   - Choose randomly 20 sequences from the MSA.
   - Initialize model parameters $\{h, J\}$ to zero.
2. **Learning:** Loop over 100000 Monte Carlo sweeps. For each sweep:
   - Loop over the 20 sequences. For each sequence $k$:
     - Loop over nucleotide of each sequence. For each nucleotide $i$:
       * Propose a new random nucleotide at position $i$
       * Compute the acceptance as $\alpha = \left(1, \frac{P_{new}}{P_{old}}\right)$, where $P_{new}$ and $P_{old}$ are the probabilities of old and new nucleotides at position $i$ according to model parameters $\{h, J\}$.
       * Accept/reject comparing $\alpha$ with a uniform random number in $[0, 1)$.
     - Compute frequencies on the 20 sequences.
   - Update parameters $\{h, J\}$ estimating likelihood gradient based on current frequences.
3. **Validation:** Repeat step 2 using parameters $\{h, J\}$ computed as averages over the last 5000 Monte Carlo sweeps of step 2.

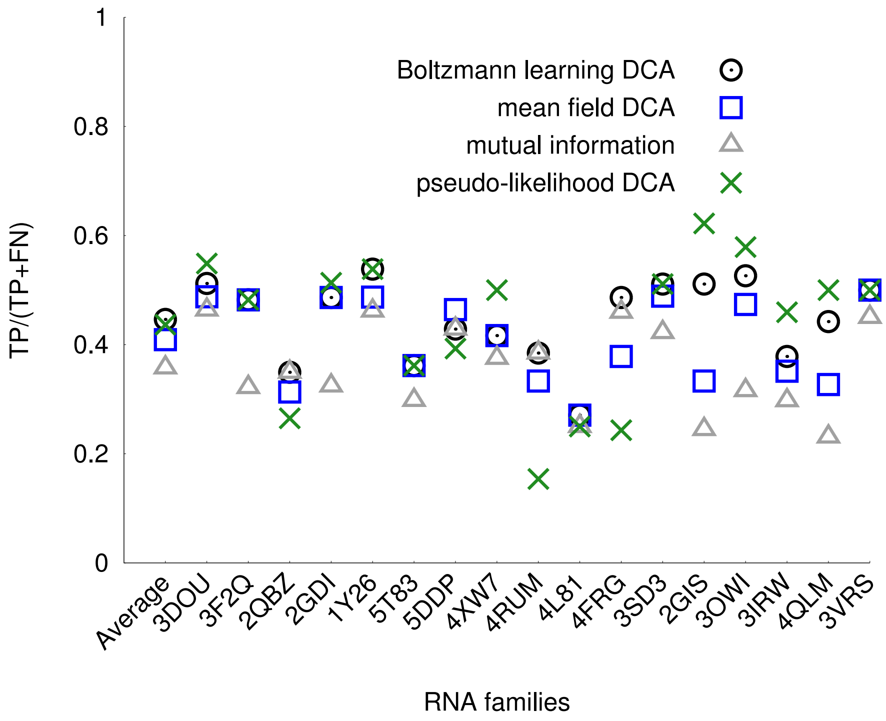


Figure 1: Sensitivity of Boltzmann learning DCA, pseudo-likelihood DCA, mean-field DCA and mutual information for all RNA families. Families are labeled using the PDB code of the representative crystallographic structure. Average sensitivity is also reported.

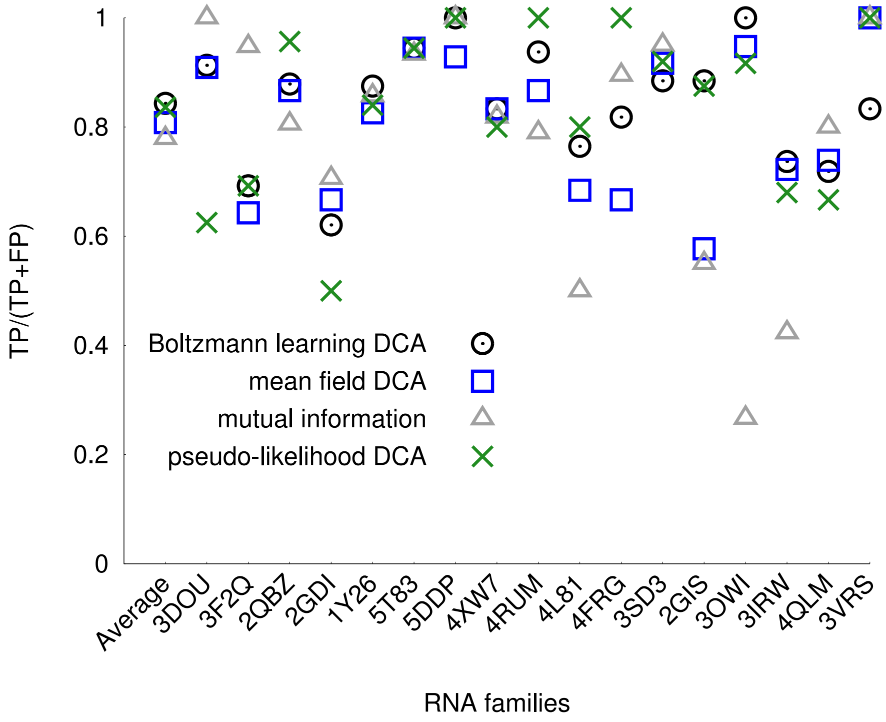


Figure 2: Precision of Boltzmann learning DCA, pseudo-likelihood DCA, mean-field DCA and mutual information for all RNA families. Families are labeled using the PDB code of the representative crystallographic structure. Average precision is also reported.

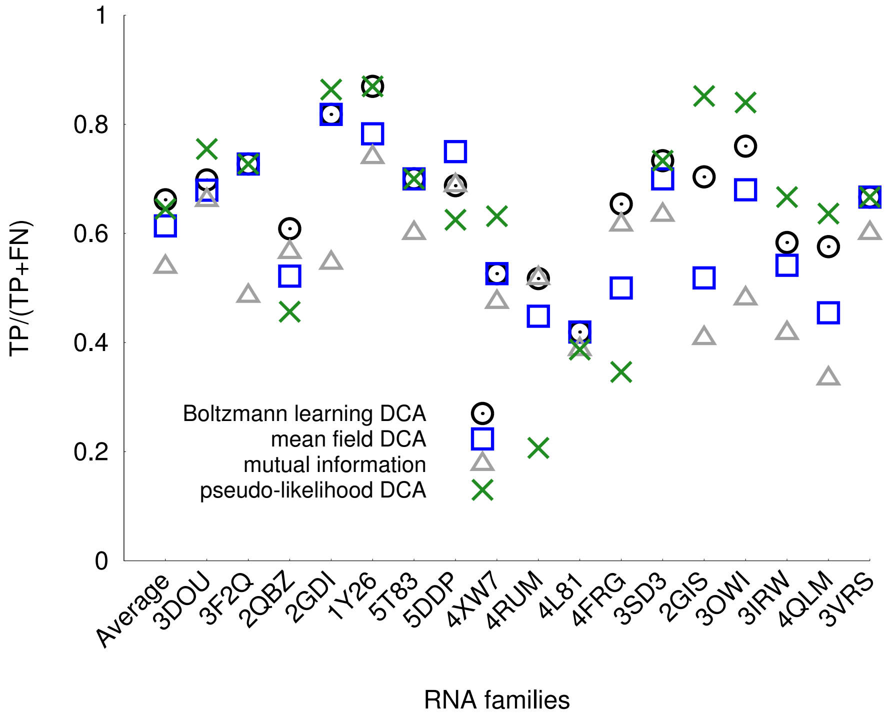


Figure 3: Sensitivity to contacts in stems (RNA secondary structure) of Boltzmann learning DCA, mean field DCA and mutual information for all families.

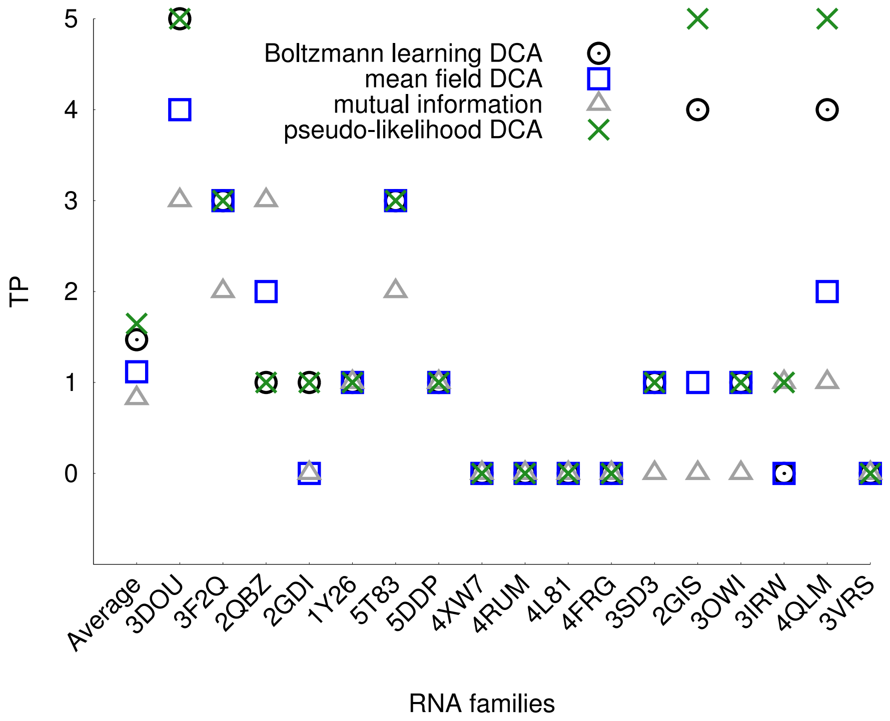


Figure 4: Number of correctly predicted (True Positives) tertiary contacts of Boltzmann learning DCA, mean field DCA and mutual information for all RNA families.

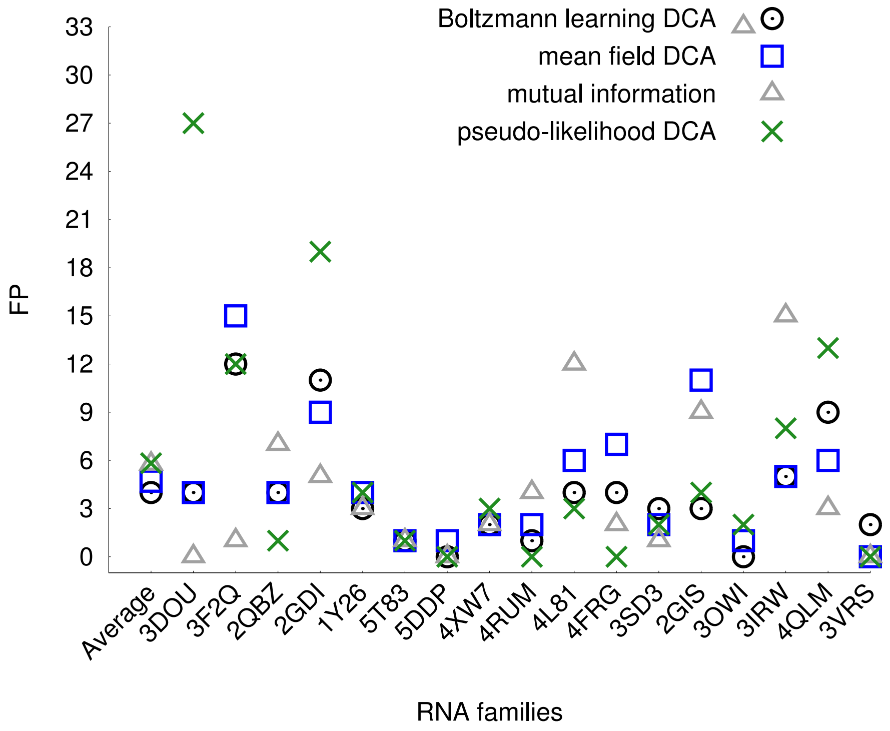


Figure 5: Number of incorrect predictions (False Positives) of Boltzmann learning DCA, pseudo-likelihood DCA, mean-field DCA and mutual information for all RNA families.Families are labeled using the PDB code of the representative crystallographic structure. Average precision is also reported.

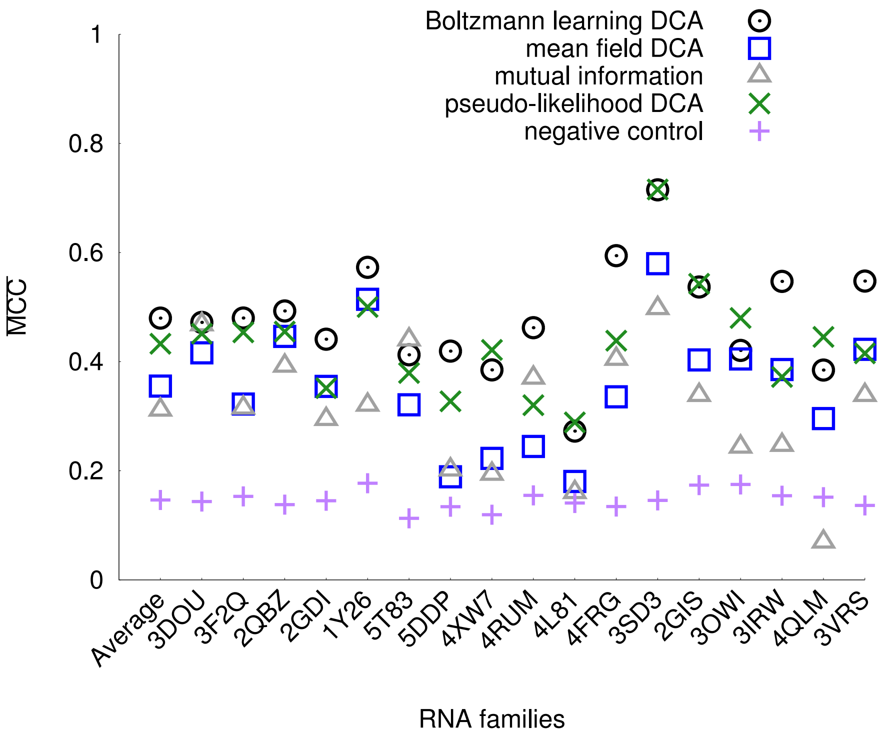


Figure 6: Clustal alignment. $\overline{MCC}$ of Boltzmann learning DCA, pseudo-likelihood DCA, mean-field DCA, mutual information for 17 RNA families at the threshold obtained through cross-validation procedure. Families are labeled using the PDB code of the representative crystallographic structure. Average $\overline{MCC}$ is also reported. Alignments are performed with *Infernal*.

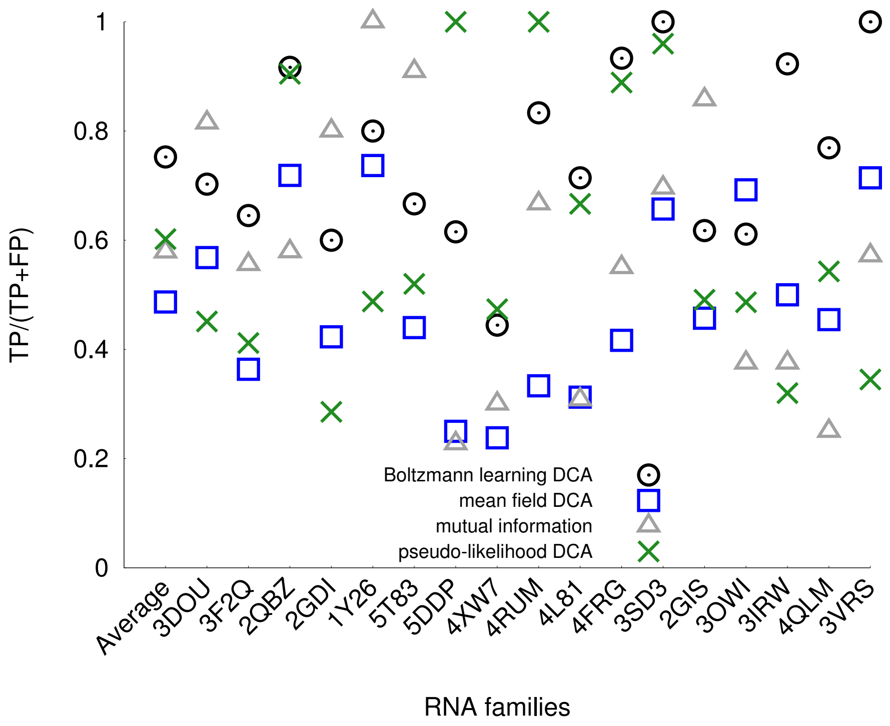


Figure 7: Clustal alignment. Precision of Boltzmann learning DCA, pseudo-likelihood DCA, mean-field DCA and mutual information for all RNA families. Families are labeled using the PDB code of the representative crystallographic structure. Average precision is also reported.

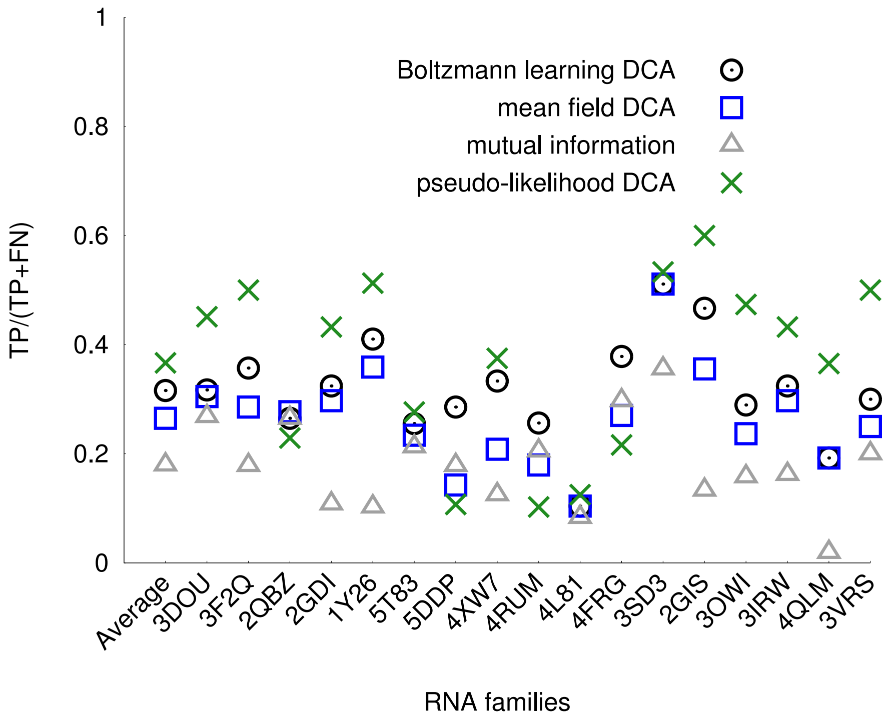


Figure 8: Clustal alignment. Sensitivity of Boltzmann learning DCA, pseudo-likelihood DCA, mean-field DCA and mutual information for all RNA families. Families are labeled using the PDB code of the representative crystallographic structure. Average sensitivity is also reported.

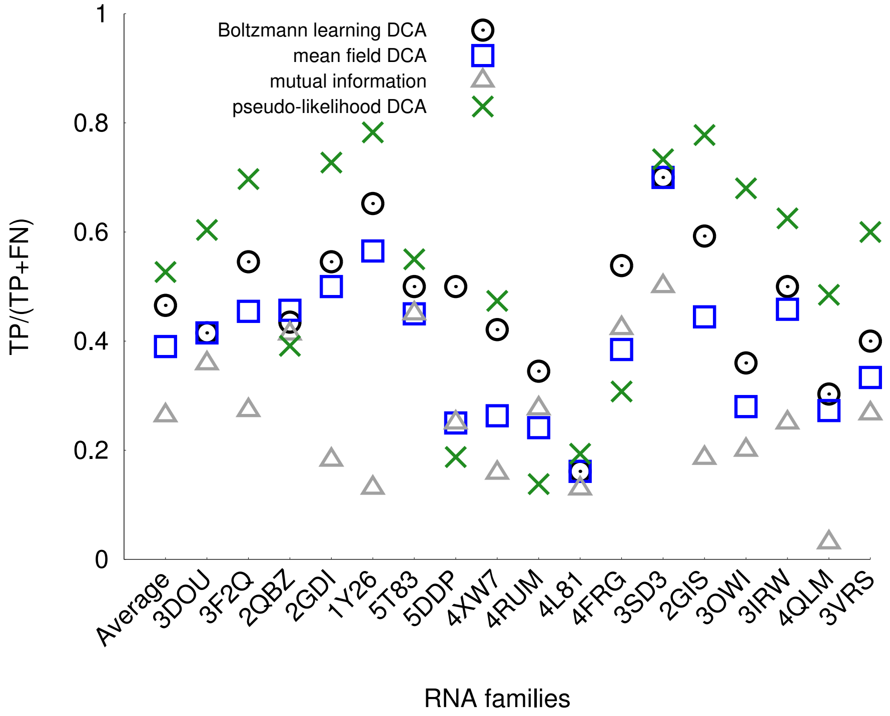


Figure 9: Clustal alignment. Sensitivity to contacts in stems (RNA secondary structure) of Boltzmann learning DCA, mean field DCA and mutual information for all families.

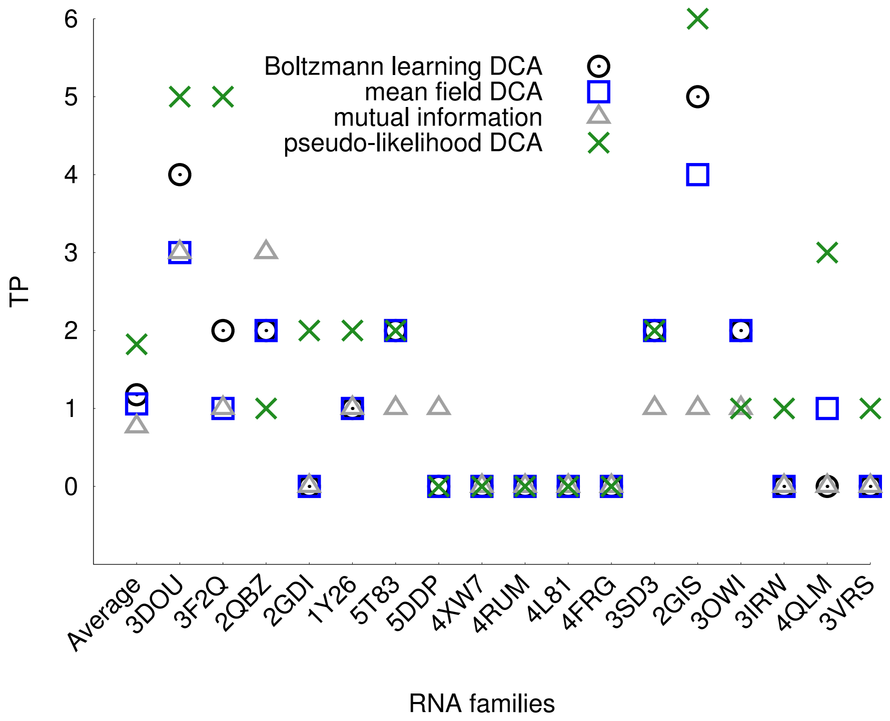


Figure 10: Clustal alignment. Number of correctly predicted (True Positives) tertiary contacts of Boltzmann learning DCA, mean field DCA and mutual information for all RNA families.

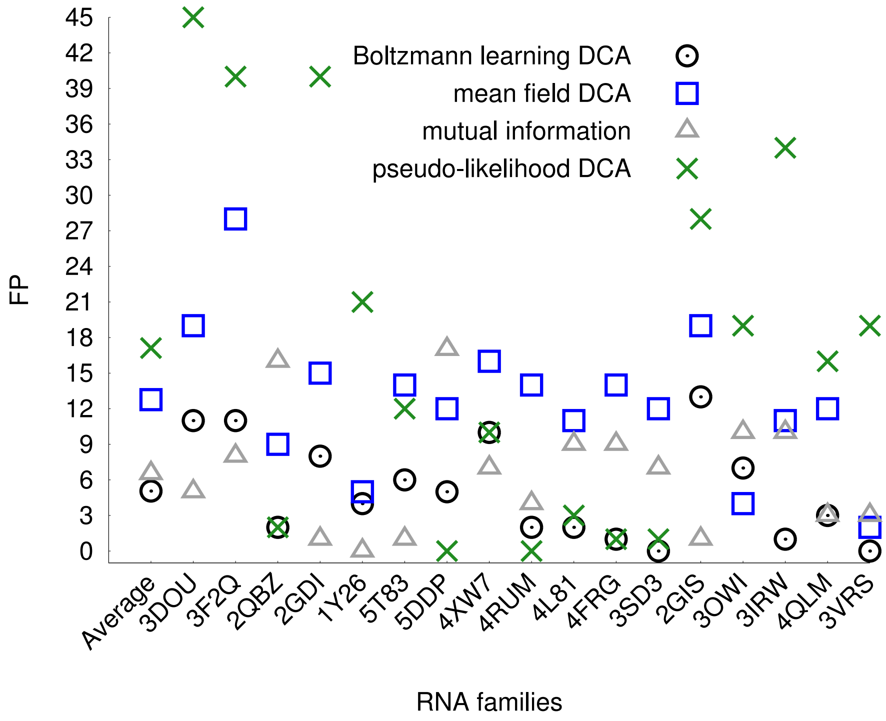


Figure 11: Clustal alignment. Number of incorrect predictions (False Positives) of Boltzmann learning DCA, pseudo-likelihood DCA, mean-field DCA and mutual information for all RNA families.Families are labeled using the PDB code of the representative crystallographic structure. Average precision is also reported.

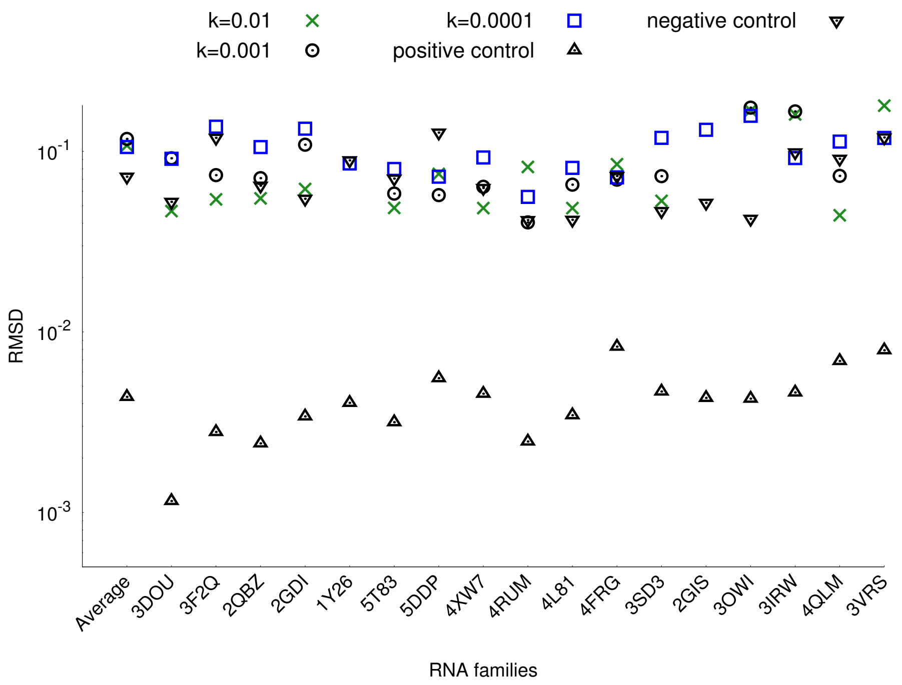


Figure 12: Validation of the coupling parameters inferred via the $l_2$-regularized pseudo-likelihood maximization method implemented at *https://github.com/magnusekeberg/plmDCA*, adopting different regularization strengths k. The validation is done running a parallel MC simulation on 20 sequences and calculating the root-mean-square deviation (RMSD) between the obtained frequencies and the empirical ones. The positive control is the statistical error due to the finite number of sequence, and the negative control is the RMSD between empirical sequences and a random sequence. Infernal alignment.

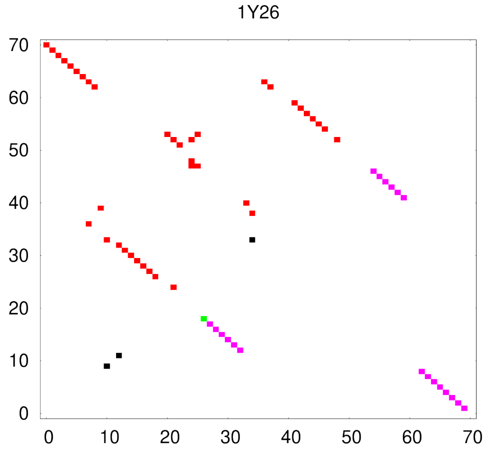


Figure 13: RF00167. Red: native structure base pairs in upper triangle. Magenta: correctly predicted secondary contacts. Green: correctly predicted tertiary contacts. Black: false positives.

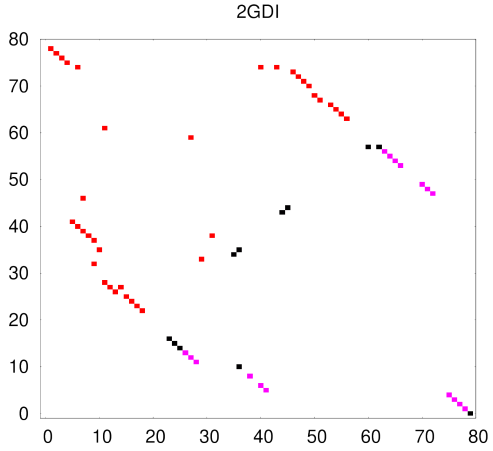


Figure 14: RF00059.Red: native structure base pairs in upper triangle. Magenta: correctly predicted secondary contacts. Green: correctly predicted tertiary contacts. Black: false positives.

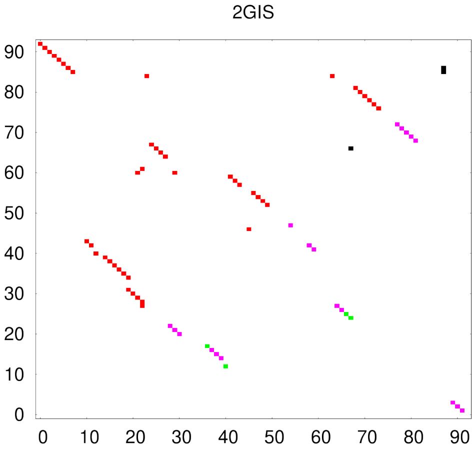


Figure 15: RF00162.Red: native structure base pairs in upper triangle. Magenta: correctly predicted secondary contacts. Green: correctly predicted tertiary contacts. Black: false positives.

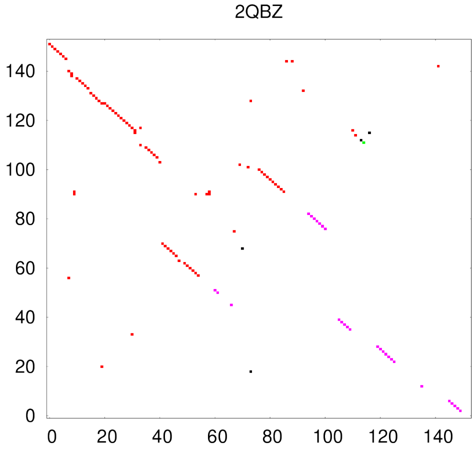


Figure 16: RF00380. Red: native structure base pairs in upper triangle. Magenta: correctly predicted secondary contacts. Green: correctly predicted tertiary contacts. Black: false positives.

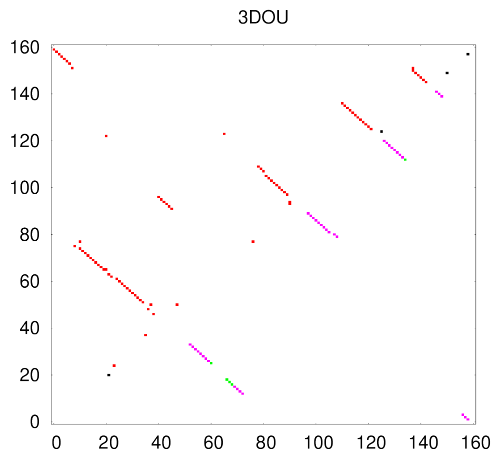


Figure 17: RF00168.Red: native structure base pairs in upper triangle. Magenta: correctly predicted secondary contacts. Green: correctly predicted tertiary contacts. Black: false positives.

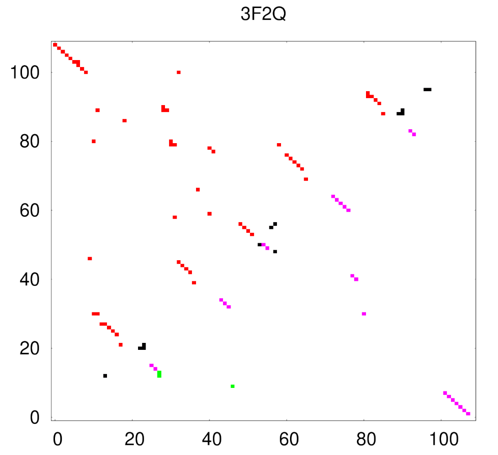


Figure 18: RF00050. Red: native structure base pairs in upper triangle. Magenta: correctly predicted secondary contacts. Green: correctly predicted tertiary contacts. Black: false positives.

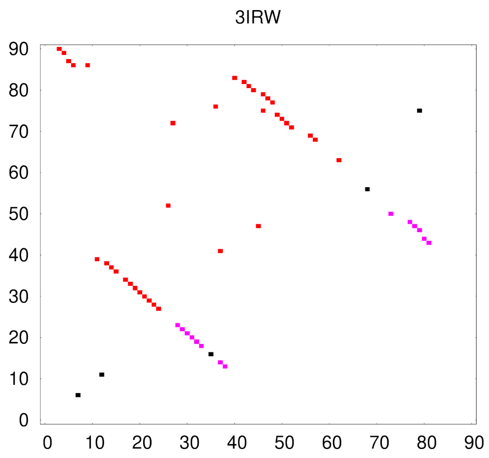


Figure 19: RF01051.Red: native structure base pairs in upper triangle. Magenta: correctly predicted secondary contacts. Green: correctly predicted tertiary contacts. Black: false positives.

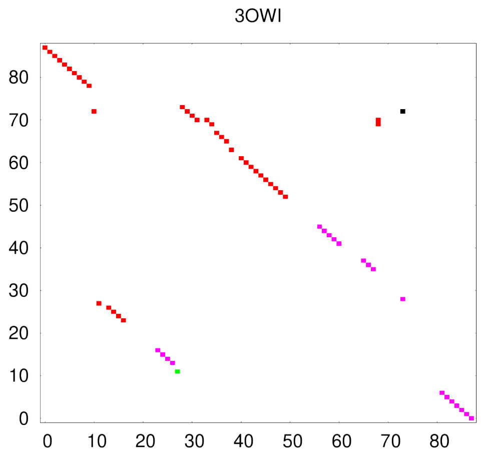


Figure 20: RF00504. Red: native structure base pairs in upper triangle. Magenta: correctly predicted secondary contacts. Green: correctly predicted tertiary contacts. Black: false positives.

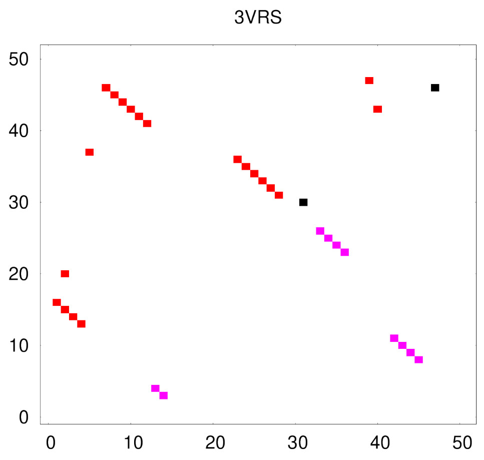


Figure 21: RF01734.Red: native structure base pairs in upper triangle. Magenta: correctly predicted secondary contacts. Green: correctly predicted tertiary contacts. Black: false positives.

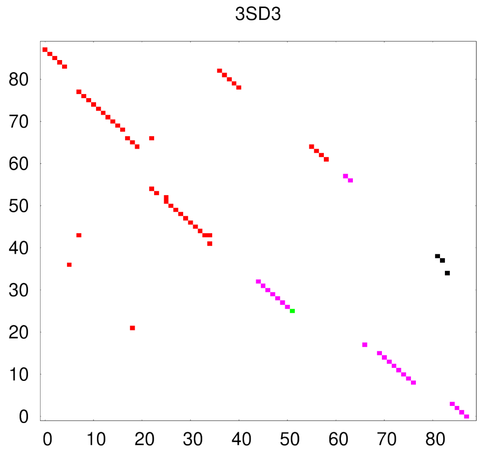


Figure 22: RF01831. Red: native structure base pairs in upper triangle. Magenta: correctly predicted secondary contacts. Green: correctly predicted tertiary contacts. Black: false positives.

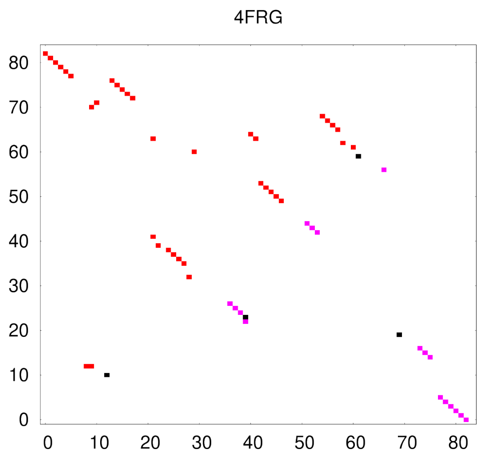


Figure 23: RF01689. Red: native structure base pairs in upper triangle. Magenta: correctly predicted secondary contacts. Green: correctly predicted tertiary contacts. Black: false positives.

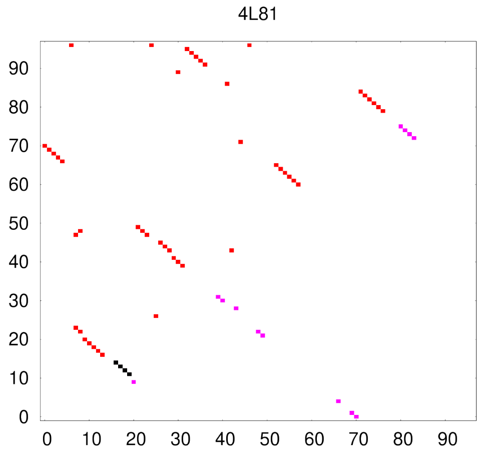


Figure 24: RF01725.Red: native structure base pairs in upper triangle. Magenta: correctly predicted secondary contacts. Green: correctly predicted tertiary contacts. Black: false positives.

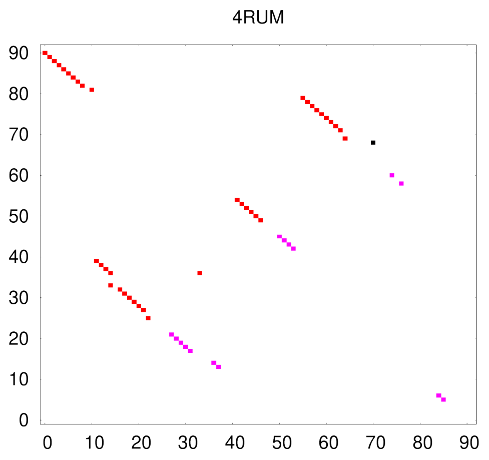


Figure 25: RF02683. Red: native structure base pairs in upper triangle. Magenta: correctly predicted secondary contacts. Green: correctly predicted tertiary contacts. Black: false positives.

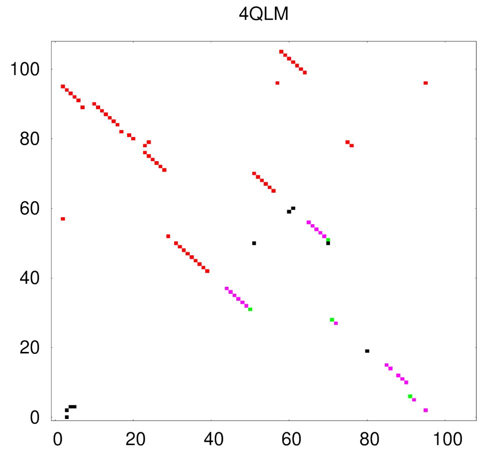


Figure 26: RF00379.Red: native structure base pairs in upper triangle. Magenta: correctly predicted secondary contacts. Green: correctly predicted tertiary contacts. Black: false positives.

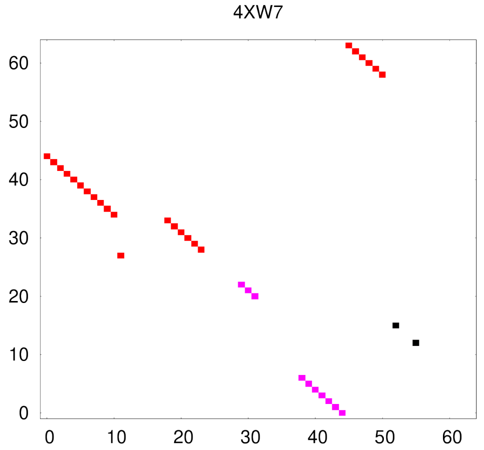


Figure 27: RF01750. Red: native structure base pairs in upper triangle. Magenta: correctly predicted secondary contacts. Green: correctly predicted tertiary contacts. Black: false positives.

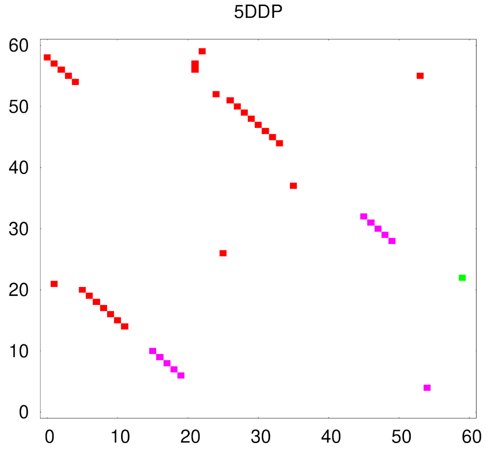


Figure 28: RF01739.Red: native structure base pairs in upper triangle. Magenta: correctly predicted secondary contacts. Green: correctly predicted tertiary contacts. Black: false positives.

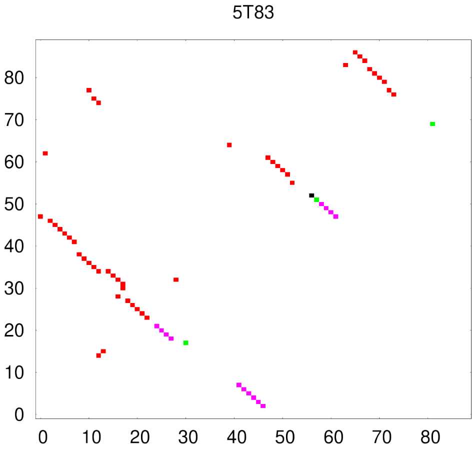


Figure 29: RF00442. Red: native structure base pairs in upper triangle. Magenta: correctly predicted secondary contacts. Green: correctly predicted tertiary contacts. Black: false positives.
